# Supplementary material for: Second virial coefficients for helium-4 and helium-3 from accurate relativistic interaction potential
Source: arXiv:2007.09767 ancillary file (2020-10-12)
Supplement: Supplementary file 1 [file supplemental.pdf]

# Supplemental information for: "Second virial coefficients for helium-4 and helium-3 from accurate relativistic interaction potential"

P. Czachorowski[1], M. Przybytek[1], M. Lesiuk[1], M. Puchalski[2], and B. Jeziorski[1]
[1] *Faculty of Chemistry, University of Warsaw, Pasteura 1, 02-093 Warsaw, Poland*
[2] *Faculty of Chemistry, Adam Mickiewicz University, Umultowska 89b, 61-614 Poznań, Poland*

(Dated: September 9, 2020)

Supplemental information consists of 7 files:

| | |
|---|---|
| `S1_data_points.txt` | calculated values of the interaction potential contributions, used to construct the analytic fits, |
| `S2_potentials.f90` | Fortran code with analytic functions fitted to the calculated data points, |
| `S3_virial_helium-3.txt` | second virial coefficient $B(T)$ and second acoustic virial coefficient $\beta_a(T)$ for helium-3 for a set of temperature values, |
| `S4_virial_helium-4.txt` | second virial coefficient $B(T)$ and second acoustic virial coefficient $\beta_a(T)$ for helium-4 for a set of temperature values, |
| `S5_SE_helium-3.txt` | calculated values of the $\mathcal{S}(E)$ function for helium-3, |
| `S6_SE_helium-4.txt` | calculated values of the $\mathcal{S}(E)$ function for helium-4, |
| `supplemental.pdf` | this file. |

### File S1_data_points.txt

The file contains recommended values (in kelvin, 1 hartree = 315775.02480407 K [1]) and estimated uncertainties of the Born-Oppenheimer interaction energy of the helium dimer, $V_{\mathrm{BO}}$, and of the adiabatic, $V_{\mathrm{ad}}$, relativistic, $V_{\mathrm{rel}}$, and QED, $V_{\mathrm{QED}}$, corrections to interaction energy. In computations we assumed mass of the helium atom nucleus $M = 7294.29954142\, m_e$ and fine structure constant $\alpha = 1/137.035999084$ [1]. All potentials are given for a set of 55 interatomic distances $1 \leq R \leq 30$ bohr. The values of $V_{\mathrm{BO}}$ for $1 \leq R \leq 9$ bohr and $V_{\mathrm{ad}}$ for all distances were taken from Ref. [2] and rescaled due to the change in the energy conversion factor (in Ref. [2] the factor 1 hartree = 315775.13 K from CODATA 2014 was used).

The file contains also our recommended values and estimated uncertainties of individual components $V_{\mathrm{CG}}$, $V_{\mathrm{D1}}$, $V_{\mathrm{D2}}$, $V_{\mathrm{Br}}$, and $V_{\mathrm{AS}}$ of $V_{\mathrm{rel}}$ and $V_{\mathrm{QED}}$

$$V_{\mathrm{rel}}(R) = V_{\mathrm{CG}}(R) + V_{\mathrm{D2}}(R) + V_{\mathrm{Br}}(R), \qquad \text{[see Eq. (53) of Ref. [3]]}, \tag{1}$$

$$V_{\mathrm{QED}}(R) = 0.037\,807\,203\, V_{\mathrm{D1}}(R) - 0.027\,938\,416\, V_{\mathrm{D2}}(R) + V_{\mathrm{AS}}(R), \qquad \text{[see Eq. (54) of Ref. [3]]}. \tag{2}$$

**File S2_potentials.f90**

The file contains code of the Fortran 2003 module `potentials_2020` that provides 15 functions:

| | |
|---|---|
| `V_BO(R)` | fit to the Born-Oppenheimer interaction energy $V_{\rm BO}$, |
| `V_AD(R)` | fit to the adiabatic correction potential $V_{\rm ad}$ for helium-4, |
| `V_REL(R)` | fit to the relativistic correction potential $V_{\rm rel}$, |
| `V_QED(R)` | fit to the QED correction potential $V_{\rm QED}$, |
| `V(R,ret,iso)` | sum of the fits to $V_{\rm BO}$, $V_{\rm ad}$, $V_{\rm rel}$, and $V_{\rm QED}$, |
| `mu2V_NA(R)` | fit to the diagonal nonadiabatic correction $\mu_n^2 V_{\rm na}^{\rm int}$, |
| `mu2Wr(R)` | fit to the rotational mass correction $\mu_n^2 \mathcal{W}_\perp^{\rm int}$, |
| `mu2Wv(R)` | fit to the vibrational mass correction $\mu_n^2 \mathcal{W}_\parallel^{\rm int}$, |
| `diff_mu2Wv(R)` | first derivative of the fit to $\mu_n^2 \mathcal{W}_\parallel^{\rm int}$, |
| `diff2_mu2Wv(R)` | second derivative of the fit to $\mu_n^2 \mathcal{W}_\parallel^{\rm int}$, |
| `sigma_BO(R)` | fit to the uncertainties of the Born-Oppenheimer energy $\sigma_{\rm BO}$, |
| `sigma_AD(R)` | fit to the uncertainties of the adiabatic correction (for helium-4) $\sigma_{\rm ad}$, |
| `sigma_REL(R)` | fit to the uncertainties of the relativistic correction $\sigma_{\rm rel}$, |
| `sigma_QED(R)` | fit to the uncertainties of the QED correction $\sigma_{\rm QED}$, |
| `sigma(R,iso)` | square root of the sum of squares of fits to $\sigma_{\rm BO}$, $\sigma_{\rm ad}$, $\sigma_{\rm rel}$, and $\sigma_{\rm QED}$, with possibility of rescaling $\sigma_{\rm ad}$ for helium-3. |

INPUT:

| | | |
|---|---|---|
| `R` | double precision | distance in bohr, |
| `ret` | logical, optional | should the retardation be switched on (`.true.`) or not (`.false.`); if not present the value `.false.` is assumed, |
| `iso` | integer, optional | isotope of helium: 3 or 4; if `iso` is not given, or `iso` is given with a value different than 3, it defaults to 4. |

OUTPUT:

| | |
|---|---|
| double precision | value of a given potential or error estimation in hartree. |

EXAMPLE:

```
use potentials_2020
write(*,*) V(5.6d0),V(5.6d0,.true.),sigma(5.6d0)
end
```

gives the result: `-3.4820795493936194E-005   -3.4820417009352500E-005   6.9992693616433796E-010`

*Notes:*

1. Analytic fits of $V_{\rm Y}(R)$, $\sigma_{\rm Y}(R)$, Y = BO, ad, rel, QED, were created in the present work. Analytic fits of $\mu_n^2 V_{\rm na}^{\rm int}(R)$ and $\mu_n^2 \mathcal{W}_{\perp/\parallel}^{\rm int}(R)$ were taken from Ref. [2].

2. In the present approach, the original fits of $\mu_n^2 \mathcal{W}_{\perp/\parallel}^{\rm int}(R)$ are used only for $R \geq 1$ bohr, as $R = 1$ bohr is the smallest distance for which these functions were calculated directly. In the region $0 \leq R \leq 1$ bohr, $\mu_n^2 \mathcal{W}_\perp^{\rm int}(R)$ and $\mu_n^2 \mathcal{W}_\parallel^{\rm int}(R)$ are approximated by third degree polynomials. The coefficients of the polynomials were obtained by imposing correct value of the functions at the origin, $\mu_n^2 \mathcal{W}_{\perp/\parallel}^{\rm int}(0) = 1/2$, and continuity of $\mu_n^2 \mathcal{W}_{\perp/\parallel}^{\rm int}(R)$ and their first and second derivatives at $R = 1$.

**File S3_virial_helium-3.txt**

The file contains the values of the second virial coefficient and the second acoustic virial coefficient for helium-3 for more temperature values than presented in the paper. It is organized as follows: temperature $T$, the second virial coefficient $B(T)$, its uncertainty $\sigma_B(T)$, the second acoustic virial coefficient $\beta_a(T)$, and its uncertainty $\sigma_{\beta_a}(T)$. All values are in cm$^3$mol$^{-1}$, except the temperature, which is in K.

**File S4_virial_helium-4.txt**

The file contains analogous data as the previous one but for helium-4.

**File S5_SE_helium-3.txt**

The file contains the value of the function $\mathcal{S}(E)$ (Eq. (10) in the paper) for helium-3, needed to calculate the thermal contribution to the second virial coefficient, $B_{\mathrm{th}}(T)$ (Eq. (8) in the paper). The columns in the file are, respectively:

1. the energy $E$ in hartree,
2. the value of $\mathcal{S}(E)$ calculated with the potential $V(R)$ (Eq. (27) in the paper),
3. the value of $\mathcal{S}(E)$ calculated with the potential $V(R)+\sigma(R)$ ($\sigma(R)$ – uncertainty of the potential),
4. the value of $\mathcal{S}(E)$ calculated with the potential $V(R)-\sigma(R)$,
5. the uncertainty $\sigma_{\mathcal{S}}(E)$ due to the ommited summation terms for $l > l_{\mathrm{max}}$ and finite propagation distance (contribution (c) described in Section IV of the paper),
6. the maximal angular momentum quantum number $l_{\mathrm{max}}$ included in the sum defining $\mathcal{S}(E)$.

The data are stored as real values except $l_{\mathrm{max}}$ – integer.

**File S6_SE_helium-4.txt**

The file contains analogous data as the previous one but for helium-4.

[1] E. Tiesinga, P. J. Mohr, D. B. Newell, and B. N. Taylor, "The 2018 CODATA Recommended Values of the Fundamental Physical Constants," (Web Version 8.1) available at http://physics.nist.gov/constants (2020).
[2] M. Przybytek, W. Cencek, B. Jeziorski, and K. Szalewicz, Phys. Rev. Lett. **119**, 123401 (2017).
[3] W. Cencek, M. Przybytek, J. Komasa, J. B. Mehl, B. Jeziorski, and K. Szalewicz, J. Chem. Phys. **136**, 224303 (2012).
